# Supplementary material for: Measuring the Measuring Tools: An Automatic Evaluation of Semantic Metrics for Text Corpora
Source: arXiv:2211.16259 source file (2022-11-29)
Supplement: Supplementary file 1 [file AppendixB.tex]

\section{Appendix}
\label{app:sdc}

\begin{figure*}[h]
    \centering
    \includegraphics[width=1\textwidth]{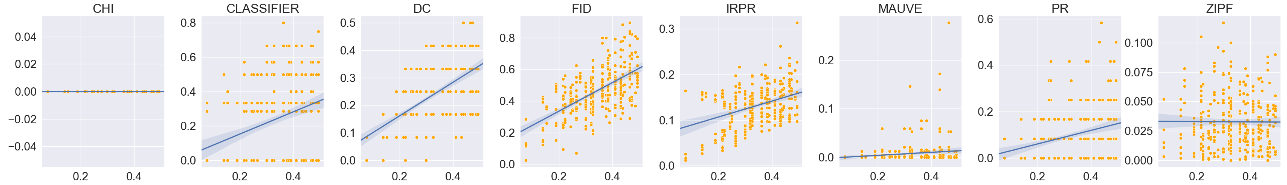}
    \caption{
    Top: Distance values (non-normalized) of corpora pairs in $(c_i,c_j)$ versus the distributional distance calculated by $(i(n-i)+j(n-j))$. ($n=k=12, |J|=6053$) where blue line indicates regression and confidence interval at 95\%. 
    Middle: Distances values calculated on increasing $s$ size corpora $a_s$ and $b_s$ sampled from sources $A$ and $B$,  correspondingly. 
    }
    \label{fig:sdc_scatter}
    
\end{figure*}

% \begin{enumerate}
%     \item define exactly what paraphrase corpora means.
%     \item Change the terminology to semantic vs non semantic.
%     \item show that non semantic is prop to j-i
%     \item Contrast between hausdroff and wassersterin.
%     \item define the distributional vs, non distributional based on the similarity to Hausdorff or wasserstein.
% \end{enumerate}

\begin{figure} [h]
    \centering
    \includegraphics[width=1\columnwidth]{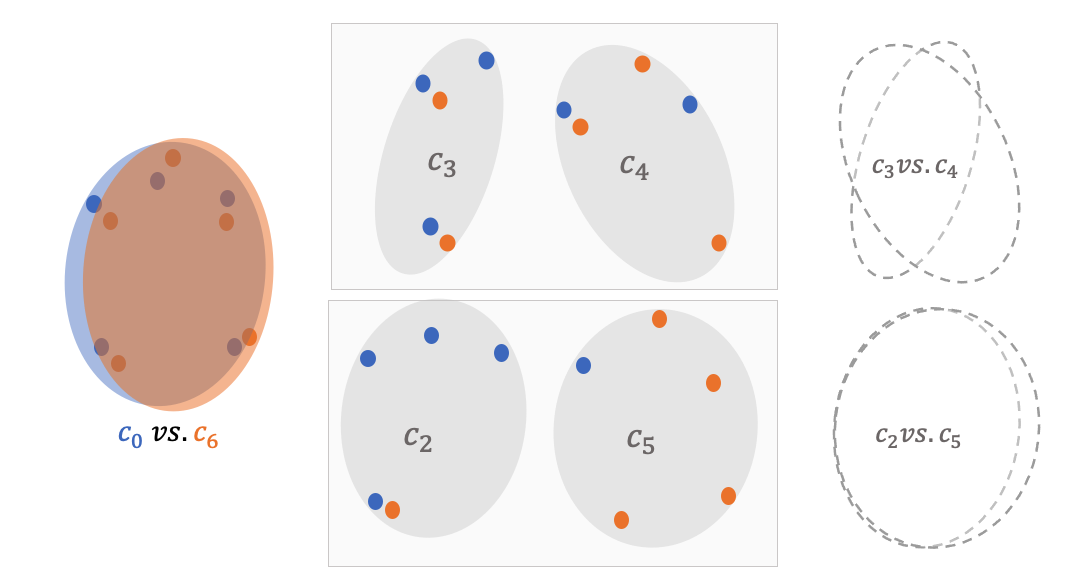}
  \caption{An illustration demonstrating the similar distribution corpora idea presented in Section \ref{sec:coverage_analysis}. 
  The distribution of the source paraphrase corpora, $C=c_1$ and $C'=c_6$ shown on the left side ($n=5$ and $k=6$). 
  In the middle panes, sample distribution $c_1$ vs. $c_5$ ($\ell=4$) and $c_3 vs. c_4$ ($\ell=1$) are shown; and the corresponding dissimilarities are demonstrated on the right. As can be seen, the larger $\ell$ is, the closer are on average $c_i$ and $c_j$ distributions (in shape and proximity). }
    \label{fig:coverage_analysis_illustration}
\end{figure}

Here we provide a proof for the intuition illustrated in Figure \ref{fig:coverage_analysis_illustration}.
We show that given a small pair of paraphrase datasets $(C,C')$ (i.e, where $n=k$), if the similarity function $d$ is \emph{distributional} then:
\begin{equation}
    d(c_i,c_j) \approx i(n-i)+j(n-j)
\end{equation}
%where $s_k(i)$ is the mapping between the indexes $(0,1,2,\dots, k)$ and its congruent palindrome indexing, i.e. $\left(0,1,2, \dots, \lfloor \frac{k}{2} \rfloor,\lfloor \frac{k}{2}+1 \rfloor, \dots, 2,1,0 \right)$.
Otherwise, if $d$ is not distributional, then $ d(c_i,c_j) \propto j-i$.
In the case of distributional metric, the distance should be proportional to the sum of the content-distances of $c_i$ to the $c_0$ and $c_j$ to $c_n$ assuming $i<j$.

This is because if $d$ is not distributional, then no special regard is given to the fact that $C$ and $C'$ are two paraphrase corpora.

\subsection{The probability for unique elements in double lottery}
Given a multiset $S^{(i)}$ containing $n$ items (non-unique), constructed by two independent sampling without replacements of $i$ ($0 \leq i \leq n$) and  $n-i$ items from  $C=\{1,2, \dots, n \}$, respectively.
We refer to this procedure the \emph{double lottery}\footnote{Eitan - here we assume that the to data set of of which is a paraphrasing of the other are very close in the embedding so that effectively we can treat them as one data set C.  We then procedure to analyse and create statistical expectation of the behaviour of quality measures under that assumption.}.
We denote the number of unique items in $S^{(i)}$, as $|S^{(i)}|$.
In addition, we denote the set of items sampled in the first sampling and the set of items sampled in the second sampling by $S_1$ and $S_2$, respectively (i.e., $S^{(i)}=S_1 \bigcup S_2$)\footnote{Eitan - better to define $S_1$ as $S^i_1$, same goes for $S_2$}. 

Let $|S^{(i)} \bigcap S^{(j)}|$ be the number of unique elements in common to $S^{(i)}$ and $S^{(j)}$.  We can model the distribution of this intersection size by modeling the number of unique elements in each of $S^{(i)}$ and $S^{(j)}$, which are determined independently.

Let $X = RSWOR(A, r)$ mean $X$ is a resulting set of $r$ random draw without replacement from a set $A$.
Let $S^{(j)}$ be formed as follows:  First draw a sample $S_1^{(j)}$ and $S_2^{(j)}$ of sizes $j$ and $n-j$ respectively, where each sample is without replacement from $C$.  That is, $S_1^{(j)}=RSWOR(C, j)$ and $S_2^{(j)}=RSWOR(C, n-j)$.  That means, in each of $S_1^{(j)}$ and $S_2^{(j)}$, the values must all be unique, but there may be shared elements (duplicates) between them. 
$S^{(i)}$ is formed the same way, of samples $S_1^{(i)}$ and $S_2^{(i)}$, except with the samples being of size $i$ and $n-i$.  For the purposes of modeling the intersection, we are interested in modeling $U_i$ and $U_j$, the number of unique items in each of $S^{(i)}$ and $S^{(j)}$.
Because sampling is done without replacement, we use the hypergeometric probability distribution.

The hypergeometric distribution is described as such. 
Say there is a collection of $N$ items (e.g., balls in a basket) of which $M\in\{0,\dots,N\}$ are of type 1 (say, black balls) and the remaining $N-M$ are of type 2 (say, white balls). 
$r\in\{0,\dots,N\}$ items are drawn without replacement from the $N$.
If the random variable $X\sim\mathcal{H}(N, M, r)$ follows the hypergeometric distribution, it models $P(X=x)$, the probability that out of the $r$ items, $x$ will be of type 1.
For instance, since the draws are without replacement (unlike a binomial random variable), $P(X=x)=0$ for $x>\textrm{min}(r,M)$, since one cannot select more items of type 1 than exist ($M$)\footnote{Eitan - or more than the number that was chosen r.}.  
A hypergeometric variable has probability mass function:
\begin{equation}
   P(X=x;N,M,r)=\frac{{M\choose x}{N-M\choose r-x}}{{N\choose r}} 
\end{equation}
and $E(X)=\frac{rM}{N}$.

In each of $S^{(i)}$ and $S^{(j)}$\footnote{Eitan - describing only for one index $S^{i}$ will carry the same message and simplify the presentation.}, let $X_i$ and $X_j$ be the number of items in the corresponding lottery sample $S_1$ (of size $i$ or $j$) that  also appear in $S_2$ (of size $n-i$ and $n-j$); that is, the size of the intersection of $S_1$ and $S_2$. 
$X_i$ can be modeled as a hypergeometric variable because out of the $N=n$ items, $M=n-i$ (or $n-j$) are of type 1 (that is, the unique items in $S_2$), and $S_1$ consists of a random with replacement of size $r=i$ (or $j$) from the $N=n$.
The number of items ($x$) out of the $r$ that are of type 1 is the size of the intersection\footnote{Eitan - Here you can either assume that n-j are fixed and you make j choices and want to determine how many of them are taken from the n-j fixed fixed choices or vice versa hence the hypergeometric distribution.}.
So $X_i\sim\mathcal{H}(n,n-i,i)$ and $X_j\sim\mathcal{H}(n,n-j,j)$, and they are independent.

If $X_i=x$, then $S^{(i)}$ consists of $n-i$ items in $S_2$, and $i$ ($=r$) items in $S_1$, of which $x$ already exist in $S_2$.  
Thus there are $(n-i)+(i-x)=n-x$ unique items in $S^{(i)}$\footnote{Eitan - Saying it differently we have chosen $n-i+i$ elements. So we have chosen $n$ elements.  $x$ of them are duplicated so we are left with $n-x$ unique elements.}, which occur with probability $P(X_i=x)$. 
Let $U_i=n-X_i$ and $U_j=n-X_j$ denote the number of unique values in $S^{(i)}$ and $S^{(j)}$. 
They have the following probabilities (the same as the hypergeometric):
\begin{equation}
    P(U_i=u_i=n-x)=\frac{{n-i\choose x}{i\choose i-x}}{{n\choose i}}=\frac{{n-i\choose n-u_i}{i\choose i+u_i-n}}{{n\choose i}}
\end{equation}
And similarly for $P(U_j=u_j)$.\\
Note that $P(U_i<max(i,n-i))=0$; and also $P(U_i)=P(U_{n-i})$. 
\begin{proof}
\begin{equation}
\begin{split}
    P(U_{n-i}=u)&=\frac{{n-n+i\choose n-u}{n-i\choose n-i+u-n}}{{n\choose n-i}}=\frac{{i\choose n-u}{n-i\choose u-i}}{{n\choose n-i}}\\
    &\underset{*}{=}
    \frac{{i\choose i-n+u}{n-i\choose n-u}}{{n\choose i}}=P(U_i=u)
\end{split}
\end{equation}
where transition $*$ employs the Binomial coefficient identity ${n \choose k} = {n \choose n-k}$.
\end{proof}

The expected value of unique number of items in $S^{(i)}$ is 
\begin{equation}
    E(U_i)=n-\frac{i(n-i)}{n}=E(U_{n-i})
\end{equation}
thus, $E(U_i)$\footnote{Eitan - Maybe say $E(U_i)$ as a function of i when i assumes values in R.} is a symmetric function around $n/2$ in which it obtain its minimum.

Now, let $Z_{ij}=|S^{(i)}\bigcap S^{(j)}|$.  
$Z_{ij}$ can also be modeled as hypergeometric for the same reason.
Say $S^{(j)}$ has $u_j$ unique elements out of $n$, and $S^{(i)}$ similarly has $u_i$ unique elements, but we do not know which ones they are. 
%However, since there are only $n$ unique elements, then when $u_i$ and $u_j$ are high, the intersection is likely to also be large (since the sets of unique elements will have to overlap).  
%And since $S^{(i)}$ and $S^{(j)}$ are formed of double lotteries, the number of unique elements in them cannot be very low, since the sampling is without replacement.  

Following the same logic as before, for fixed values $u_i$ and $u_j$, the intersection size $Z_{ij}$ will have the distribution $Z\sim H(N=n,M=u_j,r=u_i)$.

% [Note that as expected: $H(n,u_j,u_i)=H(n,u_i,u_j)$ ]

Because this distribution is conditional, and because of the independence of $U_j$ and $U_i$
\begin{equation}
\begin{split}
    P(Z_{ij}=z&, U_i=u_i, U_j=u_j)\\
    &=\frac{{u_j\choose z}{n-u_j\choose u_i-z}}{{n\choose u_i}} P(u_i) P(u_j)
\end{split}
\end{equation}
To find the overall intersection distribution (since $U_i$ and $U_j$ are random variables), we sum across all possible values, so

\begin{equation}
\begin{split}
    P(&Z_{ij}=z)= \sum_{u_i=0}^n\sum_{u_j=0}^n P(z, u_i, u_j)\\
    &= \sum_{u_i=0}^n\sum_{u_j=0}^n \left[\frac{{u_j\choose z}{n-u_j\choose u_i-x}}{{n\choose u_i}} P(U_i=u_i) P(U_j=u_j) \right]
\end{split}
\end{equation}

Figure~\ref{fig:intersection_distribution} shows the distribution of $Z^*=Z/n$\footnote{Eitan - the variable Z is not defined.  You probably mean $Z_{ij}$}, the fractional intersection size, for an example $n=10$ and $j=2$, for varying $i$.  The vertical red lines show the expected values.\footnote{Eitan - you need to calculate $E[z\mid u_i,u_j]$ prior to the following calcuation. }

\begin{equation}
\begin{split}
    E&(Z_{ij})=E(E(Z_{ij}\mid U_i,U_j))
    \\ 
    &=\sum_{u_i} \sum_{u_j} \sum_z z P(z\mid u_i,u_j) P(u_i)P(u_j)\\
    &=\sum_{u_i} P(u_i) \sum_{u_j} P(u_j) \sum_z z P(z\mid u_i,u_j) \\
    &=\sum_{u_i} P(u_i) \sum_{u_j} P(u_j) E[z\mid u_i,u_j] \\
    &=\sum_{u_i} P(u_i) \sum_{u_j} P(u_j) \frac{u_i u_j}{n} \\
    &=\sum_{u_i} u_i P(u_i) \sum_{u_j} u_j P(u_j) \frac{1}{n} \\
    &=E[U_i] E[U_j] \frac{1}{n} \\
    &=\frac{1}{n}\left[n-\frac{i(n-i)}{n}\right]\left[n-\frac{j(n-j)}{n}\right]\\
    &=\frac{1}{n}\left[n^2-i(n-i)-j(n-j)+\frac{ij(n-i)(n-j)}{n^2}\right]\\
    &=n-\frac{1}{n}\left[i(n-i)+j(n-j)-\frac{ij(n-i)(n-j)}{n^2}\right]
\end{split}
\end{equation}

% \begin{equation}
% \begin{split}
%     E(Z_{ij})&=\sum_z zP(z)\\
%     &=\sum_z z \sum_{u_i} \sum_{u_j} P(z|u_i,u_j) P(u_i)P(u_j)\\ 
%     &=\sum_{u_i} \sum_{u_j} \sum_z z P(z|u_i,u_j) P(u_i)P(u_j)\\
%     &=\sum_{u_i} P(u_i) \sum_{u_j} P(u_j) \sum_z z P(z|u_i,u_j) \\
%     &=\sum_{u_i} P(u_i) \sum_{u_j} P(u_j) E[z|u_i,u_j] \\
%     &=\sum_{u_i} P(u_i) \sum_{u_j} P(u_j) \frac{u_i u_j}{n} \\
%     &=\sum_{u_i} u_i P(u_i) \sum_{u_j} u_j P(u_j) \frac{1}{n} \\
%     &=E[u_i] E[u_j] \frac{1}{n} \\
%     &=\frac{1}{n}\left[n-\frac{i(n-i)}{n}\right]\left[n-\frac{j(n-j)}{n}\right]\\
%     &=\frac{1}{n}\left[n^2-i(n-i)-j(n-j)+\frac{ij(n-i)(n-j)}{n^2}\right]\\
%     &=n-\frac{1}{n}\left[i(n-i)+j(n-j)-\frac{ij(n-i)(n-j)}{n^2}\right]
% \end{split}
% \end{equation}

\noindent
Thus, in the case of similar distribution corpora, the distance between the two corpora $c_i$ and $c_j$ is proportional the number of shared items between $c_i$ and $c_j$, expect of the fact that $c_i$ and $c_j$ are sampled from pairs if synonym corpora, 
\begin{equation}
\begin{split}
    d(c_i,c_j)&\propto 1- \frac{E(|S^{(i)} \bigcap S^{(j)}|)}{n}\\
    &=1-\frac{E(Z_{ij})}{n}\\
    &=\frac{1}{n^2}\left[i(n-i)+j(n-j)-\frac{ij(n-i)(n-j)}{n^2}\right]\\
    &\approx \frac{1}{n^2}\left[i(n-i)+j(n-j)\right]\\
    &\propto i(n-i)+j(n-j)
\end{split}
\end{equation}

\begin{figure*}
    \centering
    \includegraphics[width=0.85\textwidth]{LaTeX/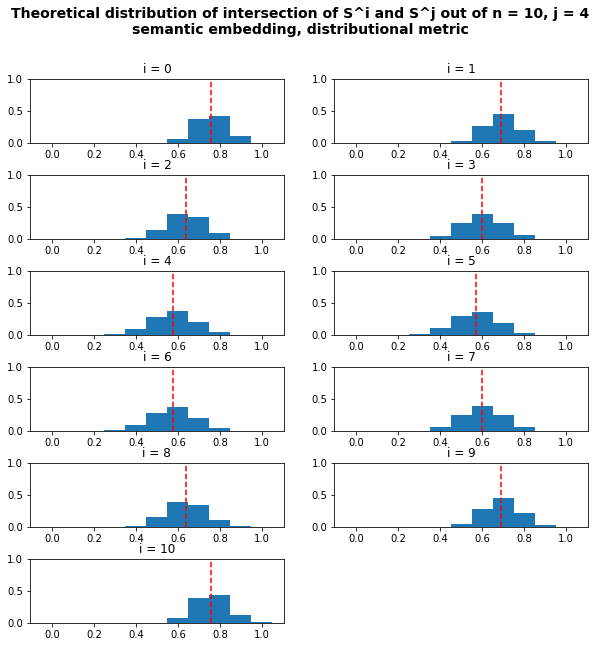}
   \caption{Distribution of fractional intersection size $Z^*=Z/n$, for $n=10$ and $j=2$.  The distributions are identical for pairs $i$ and $n-i$.  The vertical red lines show the distribution expected value.}
    \label{fig:intersection_distribution}
\end{figure*}

\iffalse

\subsection{The probability for unique elements in double lottery} 

\emph{Basically, we want to calculate the expected value of common items between two double-lottery selections given $i$ and $j$, namely, $E\left\{|S^{(i)} \bigcap S^{(j)}|\right\}$}.

In the following we calculate the probability for  $|S^{(i)}| \geq w$.
Obviously, $P(|S^{(i)}| \leq i)=1$, however, the probability of selecting at least $v$ different items out of the $n-i$ items not in $S_1$: 
\begin{equation}
   P(|S_2 \setminus S_1| \geq v )=\frac{n-i}{n}\cdot \frac{n-1-i}{n-1} \cdot \dots \cdot \frac{n+1-v-i}{n+1-v} = 
   \frac{(n-v)!}{n!}\frac{(n-i)!}{(n-i-v)!}=\frac{(n-i)_v}{(n)_v}
\end{equation}
Namely, the probability is equal to the number of variations of $v$ items out of all the remaining $n-i$ items divided the number of combinations for selecting $v$ items out of $n$ items.
Note that $P(|S_2 \setminus S_1| \geq 1 )=\frac{n-i}{n}$, i.e., the probability of selecting an item from $S$ which is not in $S_1$.

For ease of notation, let us denote by $m_{i,n}$ the random variable representing $|S^{(i)}|$ and $\alpha_{i,n}=max(i, n-i)$.
Therefore, the probability that $m_{i,n} \geq w$ is as follows:

\begin{equation}
   P(m_{i,n} \geq w) \begin{cases}
  1 & \text{if $w \leq \alpha_{i,n}$} \\
  \frac{(n-\alpha_{i,n})_{w-\alpha_{i,n}}}{\binom{n}{w-\alpha_{i,n}}} & \text{otherwise}
\end{cases}
\end{equation}
$P(m_{i,n} \geq w)$ is the probability that $c_i$ contains at least $w$ different items.
\fi

\subsection{Embeddings and distribution type}

Let $C$ and $C'$ be two paraphrase corpora of the same size $n$, where item indexed $i$ in $A$ corresponds\footnote{Eitan - I think it corresponds through paraphrasing.  If correct let us make it explicit.} to the same index in $B$.  We have distinguished between distance functions $d$ that are \emph{distributional} and those that are \emph{non-distributional}.  Furthermore, the embedding technique can be considered to be \emph{semantic} or not.  \footnote{Eitan - define or at least give an example for semantic and not semantic.  One possible simple definition we can use follows.  An embedding is $\delta$ semantic if there exist a distance measure d(x, y) over the embedding space so that if x and y are a paraphrasing pair then d(x, y) is less than some pre defined $\delta$.  Can we say cosine similarity instead of a distance?} Let the notation $a\sim b$ mean that $a$ and $b$ are paraphrases of each other, meaning they are natural language utterances with the same effective meaning but use different words.  In paraphrase corpora, $\forall i=1,\dots,n$, if $a\in C$ and $b\in C'$ are each the $\nth{i}$ indexed item, then $a\sim b$.  This means that if the embedding used on $a$ and $b$ is \emph{semantic} (i.e., accounts for the overall meaning of the words, even if the words do not overlap, such as word2vec), $a$ and $b$ should be close in the embedding space.  If the embedding is \textit{non-semantic} (e.g., term or $n$-gram frequency embedding, which captures only the frequencies of the actual words or letter combinations used and not their semantic meaning), then $a$ and $b$ should\footnote{Eitan - change should to may.} not be particularly close to each other in the embedded space; more specifically, we will assume in the idealized case that $a$ and $b$ are no closer to each other than they are to other members of $C$ and $C'$.

Consider a distance metric $\delta(x,y)=1-I(x= y)$; that is, identical items $x,y$ ($I(x=y)=1$)\footnote{Eitan - do you mean identical or $a\sim b$ a paraphrase pair?; Sam: identical items, but a semantic embedding in this extreme will map paraphrases to the same item, while non-paraphrases will be mapped to different items} are at distance 0 from each other, and any pair where $x\ne y$ have distance 1, regardless of the actual values of $x$ and $y$.  Let us define $C_{\textrm{sem}}$ and $C'_{\textrm{sem}}$ be the respective embeddings if the embedding is semantic, and $C_{\textrm{nonsem}}$ and $C'_{\textrm{nonsem}}$ if not.  Without lack of generality, let us denote $C_{\textrm{sem}}=C'_{\textrm{sem}}=\{1,2,\dots,n\}$.  Because the corresponding elements $a\in C_{\textrm{sem}}$ and $b\in C'_{\textrm{sem}}$ have the same value, and the values within each corpus are unique, then we have $\delta(a,b)=0$ whenever $a\sim b$, otherwise $\delta(a,b)=1$.  This captures the ideal scenario in which paraphrase pairs $a,b$ have exactly 0 distance in the semantic embedded space (in reality the distance will not be exactly zero but will typically be a small value) and have maximal distance 1 from all other semantically embedded utterances in the corpus.  In contrast, if the embedding is non-semantic, then in the ideal case, $a\sim b$ should not make them closer to each other in this space.  Let us denote $C_{\textrm{nonsem}}=\{n+1,\dots,2n\}$ and $C'_{\textrm{nonsem}}=\{2n+1,\dots,3n\}$; thus, not only are the embedded values in each corpus unique, but also all values are distinct from each other (and hence have distance $\delta(a,b)=1$, even if $a\sim b$). \footnote{Eitan - let's test if TF-IDF actually has all paraphrase pairs far away.} 

\subsubsection{Non-semantic and distributional metric}

If the embedding is non-semantic, then the two source corpora do not overlap.  We form the double lottery draws $S_1^{(j)}=RSWOR(C_{\textrm{nonsem}}, j)$, $S_2^{(j)}=RSWOR(C'_{\textrm{nonsem}}, n-j)$, $S_1^{(i)}=RSWOR(C_{\textrm{nonsem}}, i)$ and $S_2^{(i)}=RSWOR(C'_{\textrm{nonsem}}, n-i)$.  Because the two nonsemantic corpora do not overlap, within each of $S^{(i)}$ and $S^{(j)}$, all elements are unique.  Hence we need only consider the probability of intersections between $S_1^{(i)}$ and $S_1^{(j)}$ (both from $C_{\textrm{nonsem}}$), and between $S_2^{(i)}$ and $S_2^{(j)}$ (both from $C'_{\textrm{nonsem}}$).  Recall all the draws are mutually independent.

Let $Z_{1,ij}=|S_1^{(i)}\bigcap S_1^{(j)}|$ and $Z_{2,ij}=|S_2^{(i)}\bigcap S_2^{(j)}|$ be the intersection sizes.  Following the earlier intuition, $Z_{1,ij}\sim \mathcal{H}(n,i,j)$ and $Z_{2,ij}\sim \mathcal{H}(n,n-i,n-j)$.  Because these are independent and the two halves cannot overlap, $|S^{(i)} \bigcap S^{(j)}|=Z_{ij}=Z_{1,ij} + Z_{2,ij}$, and so $E(Z_{ij})=E(Z_{1,ij}) + E(Z_{2,ij})=\frac{ij}{n} + \frac{(n-i)(n-j)}{n}$.  To convert this into a distance measure, we take $1-E(Z_{ij})/n=\frac{n(i+j)-2ij}{n^2}$

The distribution of $Z_{ij}$ is given as follows:

$P(Z_{ij}=z)=\sum_{a=0}^z P(a\mid N=n, M=i, r=j)\times P(n-a\mid N=n, M=n-i, r=n-j)$, where the probability is calculated by examining all possible combinations of intersection sizes on the two halves that sum to a value $z$ for $Z_{ij}$; for each, the probabilities are multiplied since they are independent events.

The distribution of $Z_{ij}/n$ is shown in Figure~\ref{fig:distributional_nonsemantic}, for $j=4$ and $n=10$.

\begin{figure*}[h]
    \centering
    \includegraphics[width=1\textwidth]{LaTeX/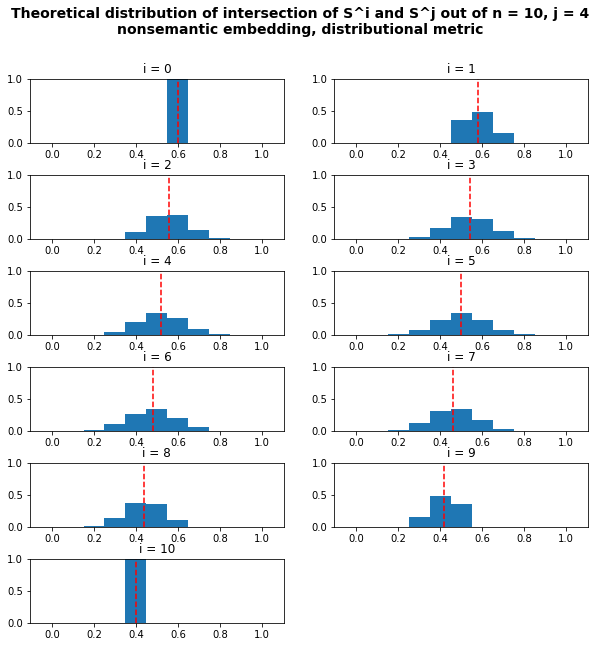}
    \caption{}
    \label{fig:distributional_nonsemantic}
\end{figure*}

Figure~\ref{fig:intersection_distributional} compares $E(Z_{ij})/n$, for $j=4$ and $n=10$ for the semantic and nonsemantic cases.  Clearly, similarity is higher in the semantic embedding.

\begin{figure*}[h]
    \centering
    \includegraphics[width=1\textwidth]{LaTeX/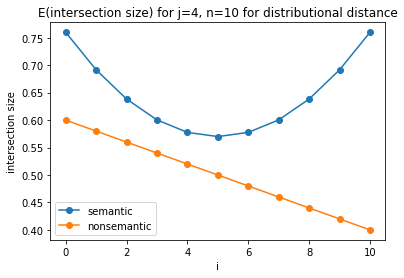}
    \caption{}
    \label{fig:intersection_distributional}
\end{figure*}

\subsubsection{Non-distributional metric}

For a non-distributional metric, we use the Average Hausdorff distance between two sets $A$ and $B$, which can consist of repeated items.  This distance is defined, for a general distance $d(a,b)$ between elements $a\in A$ and $b\in B$, as $d_{AVD}(A,B)=0.5\left(\left(\frac{1}{|A|}\sum_{a\in A}\textrm{min}_{b\in B}d(a,b)\right) + \left(\frac{1}{|B|}\sum_{b\in B}\textrm{min}_{a\in A}d(a,b)\right)\right)$.  That is, the distance to the closest item in $B$ is found for each item in $A$, and then the average minimum distance is taken; the same is done in the reverse direction, and then the two averages are averaged equally.  It is useful when $A$ and $B$ are of different sizes, since the two directional averages are weighted equally in the final average. In our case, $A=S^{(i)}$ and $B=S^{(j)}$.  
In our case, $d(a,b)=\delta(a,b)=1-I(a=b)$, and $|S^{(i)}|=|S^{(j)}|=n$, so the formula simplifies to 
\begin{equation}
\begin{split}
d_{AVD}&(A,B)=\\
&=\frac{(n - \sum_{a\in A}I(a \in B)) + (n - \sum_{b\in B}I(b \in A))}{2n}\\
&=\frac{(2n) - ((\sum_{a\in A}I(a \in B)) + (\sum_{b\in B}I(b \in A)))}{2n}\\
&=1 - \frac{(\sum_{a\in A}I(a \in B) + \sum_{b\in B}I(b \in A)}{2n}
\end{split}
\end{equation}
The similarity, rescaled by $n$, is $Z_{ij}=n(1-d_{AVD}(S^{(i)}, S^{(j)}) = \frac{(\sum_{a\in A}I(a \in B) + \sum_{b\in B}I(b \in A)}{2}$.

The simplest case is when the corpora are nonsemantic.  In this case, because the elements in each of $A$ and $B$ are unique within each set, the directional similarities are equal, and so $Z_{ij}=\sum_{a\in A}I(a \in B)=Z_{1,ij}+Z_{2,ij}$ as in the distributional non-semantic case.  Thus, $E(Z_{ij})=\frac{ij}{n} + \frac{(n-i)(n-j)}{n}$ as well.  The intuition is as such: the distributional intersection size only measures the number of unique elements shared (the set intersection), while Average Hausdorff distance, when converted to a similarity, will count duplicated items as well.  For instance, if $A = \{1,1,2,3,4\}$ and $B=\{1,2,5,6,7\}$, $A$ has 3 elements (1 counts twice) that are in $B$, while $B$ only has 2 in $A$.  The similarity will thus be $0.5((3/5)+(2/5))=0.5$, while the intersection size is only 2, or $2/5$ as a fraction. But in non-semantic corpora, the elements in each $S^{(i)}$ and $S^{(j)}$ are unique, so the intersection size and Average Hausdorff similarity are equivalent.  Thus, the non-distributional and distributional distance metrics achieve the same result in this simplified scenario.

\begin{figure*}[h]
    \centering
    \includegraphics[width=1\textwidth]{LaTeX/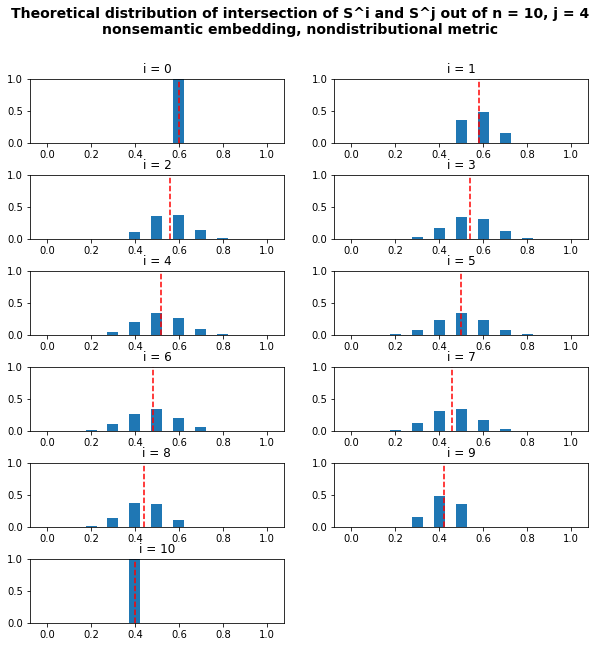}
    \caption{}
    \label{fig:nondistributional_nonsemantic}
\end{figure*}

The semantic case is more complicated.  We use the fact established earlier, that $U_i$ and $U_j$, the number of unique elements in each of $S^({i})$ and $S^{(j)}$, are distributed as $U_i\sim\mathcal{H}(n,n-i,i)$ and $U_j\sim\mathcal{H}(n,n-j,j)$, in the semantic case (in the semantic case, all values in each are unique).  
Let $k$ denote $i$ or $j$, and $\bar{k}$ denote the other value (i.e., if $k=i$, then $\bar{k}=j$, and vice versa).  Here, let $Z_{1,k}\textrm{ and } Z_{2,k},\:k=i,j$, be the number of items in $S_1^{(k)}$ and $S_2^{(k)}$ that appear in the corresponding half of the other sample $\bar{k}$.  These distributions depend on $U_i=u_i$ and $U_j=u_j$ have the distributions $Z_{1,k}\mid u_{\bar{k}}\sim \mathcal{H}(n,u_{\bar{k}},k)$ and $Z_{2,k}\mid u_{\bar{k}}\sim \mathcal{H}(n,u_{\bar{k}},n-k)$. All are mutually independent once conditioning on $u_i,u_j$ is done. $Z_{1,k}+Z_{2,k}$ are the total number of items in one sample $S^{(k)}$ (e.g., $A$ or $B$) that appear in the other ($B$ or $A$).  Thus, letting $Z_{ij}=\frac{(Z_{1,i}+Z_{2,i}) +(Z_{2,j)}+Z_{2,j})}{2}$, $Z_{ij}/n$ gives $d_{AVD}(S^{(i)}, S^{(j)})$.

The distribution can be obtained empirically through a set of convolutions ($Z_1^{(k)}$ with $Z_2^{(k)}$ to produce $Z^{(k)}$, and then a convolution of them to produce $Z_{ij}$.  Empirically, the calculation is as follows:

\begin{equation}
P(Z_{ij}=z)=\\\sum_{u_i=0}^n\sum_{u_j=0}^n\\\left(\sum_{(a,b,c,d)\colon\:a,b,c,d\in\{0,1,\dots,z\}\textrm{ and }a+b+c+d=z}\\
P(Z_1^{(i)}=a\mid u_j)P(Z_2^{(i)}=b\mid u_j)P(Z_1^{(j)}=c\mid u_i)P(Z_2^{(j)}=d\mid u_i)\right)P(U_i=u_i)P(U_j=u_j)
\end{equation}

A plot of $Z_{ij}/n$ for this case is shown in Figure~\ref{fig:nondistributional_semantic}.  Figure~\ref{fig:intersection_nondistributional} shows the relationship between expected intersection size for semantic vs nonsemantic cases for the nondistributional metric.  This is very similar to the pattern Figure~\ref{fig:intersection_distributional} 
except that in the semantic case, the similarity is slightly higher, as discussed.

\begin{figure*}[h]
    \centering
    \includegraphics[width=1\textwidth]{LaTeX/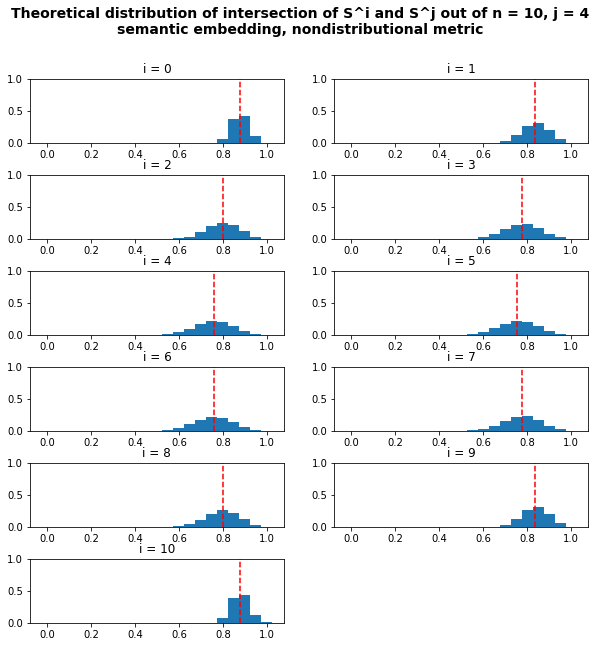}
    \caption{}
    \label{fig:nondistributional_semantic}
\end{figure*}

\begin{figure*}[h]
    \centering
    \includegraphics[width=1\textwidth]{LaTeX/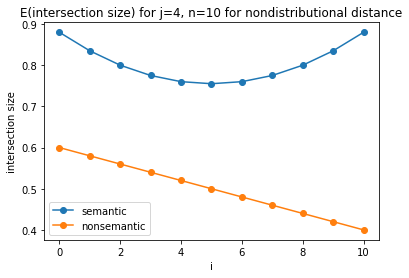}
    \caption{}
    \label{fig:intersection_nondistributional}
\end{figure*}

\subsection{Adversarial embeddings}

Consider $C_{\textrm{adv}}=\{1,\dots,n\}$ as before, and say there is a (semantic?) embedding that is adversarial in that it maps non-p
